# Supplementary material for: Orthogonal Time Frequency Space (OTFS) Modulation for Wireless Communications
Source: arXiv:2208.11807 source file (2022-08-25)
Supplement: Supplementary file 1 [file appendix.tex]

\chapter{Detailed Proofs}\label{c:literature}

Proofs.
